# Supplementary material for: Finding path and cycle counting formulae in graphs with Deep Reinforcement Learning
Source: arXiv:2410.01661 source file (2025-01-23)
Supplement: Supplementary file 1 [file supplementaryH.tex]

\section{LLM in our framework}\label{app:CFG}

The classical transformers used in practice in Large Language Models (LLM) can be implemented through our framework. Indeed, such transformers generate sentence with the following grammar

\begin{align}\label{eq:LLMgrammar}
    W \rightarrow \alpha_1 W \ | \ \cdots \ | \ \alpha_k W \ | \ \mathrm {stop}.
\end{align}
Where $\{\alpha_1, \cdots, \alpha_k \}$ is the vocabulary of the LLM. The PDA corresponding to this CFG, start with the start variable $W$, and then add a letter to the terminal symbols already generated until the terminal symbol $\mathrm {stop}$ is generated.
